# Supplementary material for: XraySyn: Realistic View Synthesis From a Single Radiograph Through CT Priors
Source: arXiv:2012.02407 source file (2022-03-24)
Supplement: Supplementary file 4 [file network_M.tex]

\begin{table}[htb!]
\centering 
\begin{tabular}{l | c | l}
Name & $N_{c}$ & Description \\
\hline
INPUT & $1$ & Input $I^{T}_{\textrm{in}}$\\ 
CONV0 & $32$ & K3-C1-S2-P1 \\
RELU &  & \\
CONV1 & $64$ & K3-C64-S2-P1 \\
RELU &  & \\
CONV2 & $128$ & K3-C64-S2-P1 \\
RELU &  & \\
CONV3 & $256$ & K3-C128-S2-P1 \\
RELU &  & \\
CONV4 & $512$ & K3-C256-S2-P1 \\
RELU &  & \\
CONV5 & $1024$ & K3-C512-S2-P1 \\
RELU &  & \\
CONV6 & $2048$ & K3-C1024-S2-P1 \\
RELU &  & \\
CONV4 & $4096$ & K3-C2048-S2-P1 \\
\midrule
\end{tabular}
\caption{Network architecture of $\mathcal{M}$ in 2DRN.}
\label{table:2DRN-M-fg}
\end{table}
