# Supplementary material for: XraySyn: Realistic View Synthesis From a Single Radiograph Through CT Priors
Source: arXiv:2012.02407 source file (2022-03-24)
Supplement: Supplementary file 6 [file tissue_weight.tex]

%& $\textrm{XraySyn}_{ref}$ 
\captionsetup[subfigure]{labelformat=empty}
\begin{figure}[htb!]
    \setlength{\abovecaptionskip}{3pt}
    \setlength{\tabcolsep}{1pt}
    \centering
    \begin{tabular}[b]{ccc}
        \begin{subfigure}[b]{0.33\linewidth}
            \includegraphics[width=\textwidth,height=\textwidth]{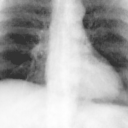}
            \caption{$\omega_{tissue}=1$}
        \end{subfigure} &
        \begin{subfigure}[b]{0.33\linewidth}
            \includegraphics[width=\textwidth,height=\textwidth]{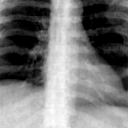}
            \caption{$\omega_{tissue}=0.7$}
        \end{subfigure}&
        \begin{subfigure}[b]{0.33\linewidth}
            \includegraphics[width=\textwidth,height=\textwidth]{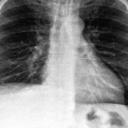}
            \caption{Input X-ray}
        \end{subfigure} \\
    \end{tabular}
    \caption{An illustration of the effect of adding a flexible weight between $\mu_{bone,E}$ and $\mu_{tissue,E}$. If no $\omega_{tissue}$ is introduced, i.e. $\omega_{tissue}=1$ always, the produced X-ray image can be very inconsistent from the input X-ray image, and with no way for adjustments.}
    \label{fig:tissue_weight}
\end{figure}
