# Supplementary material for: XraySyn: Realistic View Synthesis From a Single Radiograph Through CT Priors
Source: arXiv:2012.02407 source file (2022-03-24)
Supplement: Supplementary file 7 [file versus.tex]

%& $\textrm{XraySyn}_{ref}$ 
\captionsetup[subfigure]{labelformat=empty}
\begin{figure}[htb!]
    \setlength{\abovecaptionskip}{3pt}
    \setlength{\tabcolsep}{1pt}
    % \centering
    \begin{tabular}[b]{ccc}
        \begin{subfigure}[b]{0.33\linewidth}
            \includegraphics[width=\textwidth]{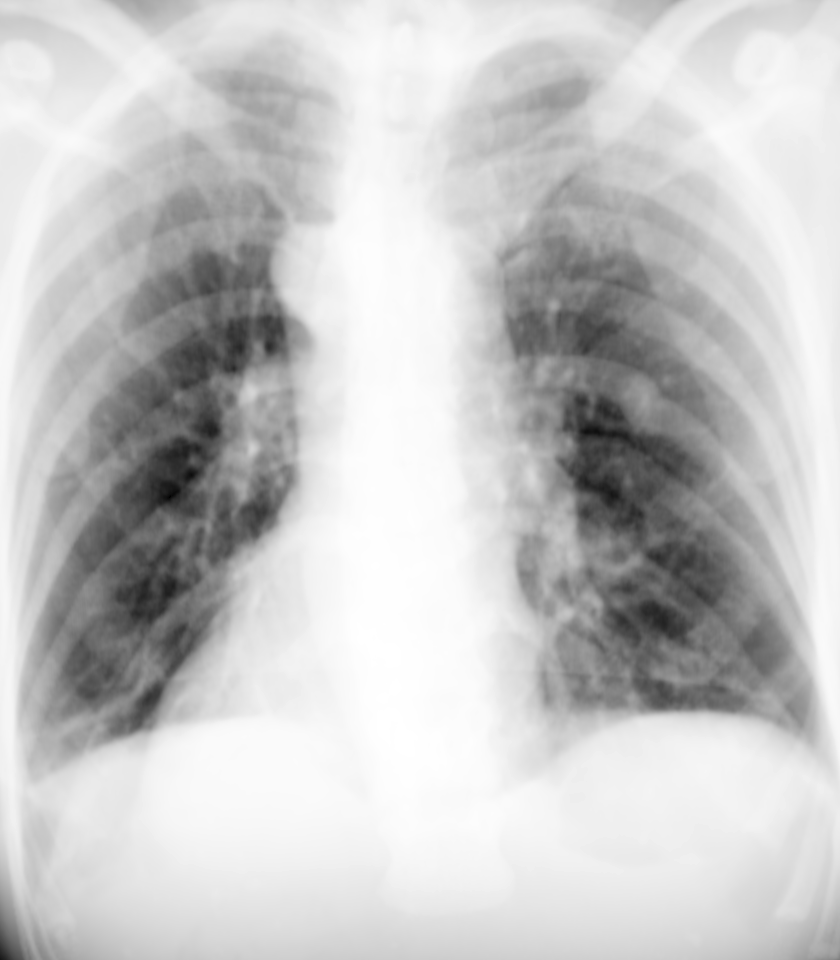}
            \caption{CT2Xray}
        \end{subfigure} &
        \begin{subfigure}[b]{0.33\linewidth}
            \includegraphics[width=\textwidth]{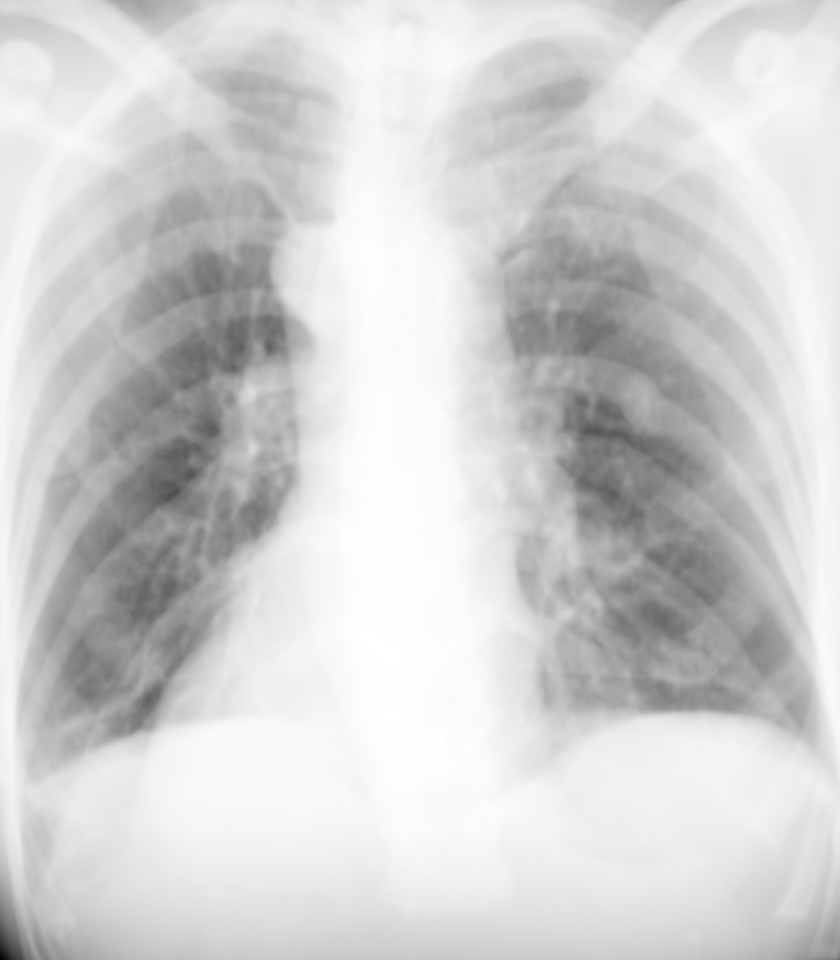}
            \caption{CT2Xray w/ $t_{air}$}
        \end{subfigure}&
        \begin{subfigure}[b]{0.33\linewidth}
            \includegraphics[width=\textwidth]{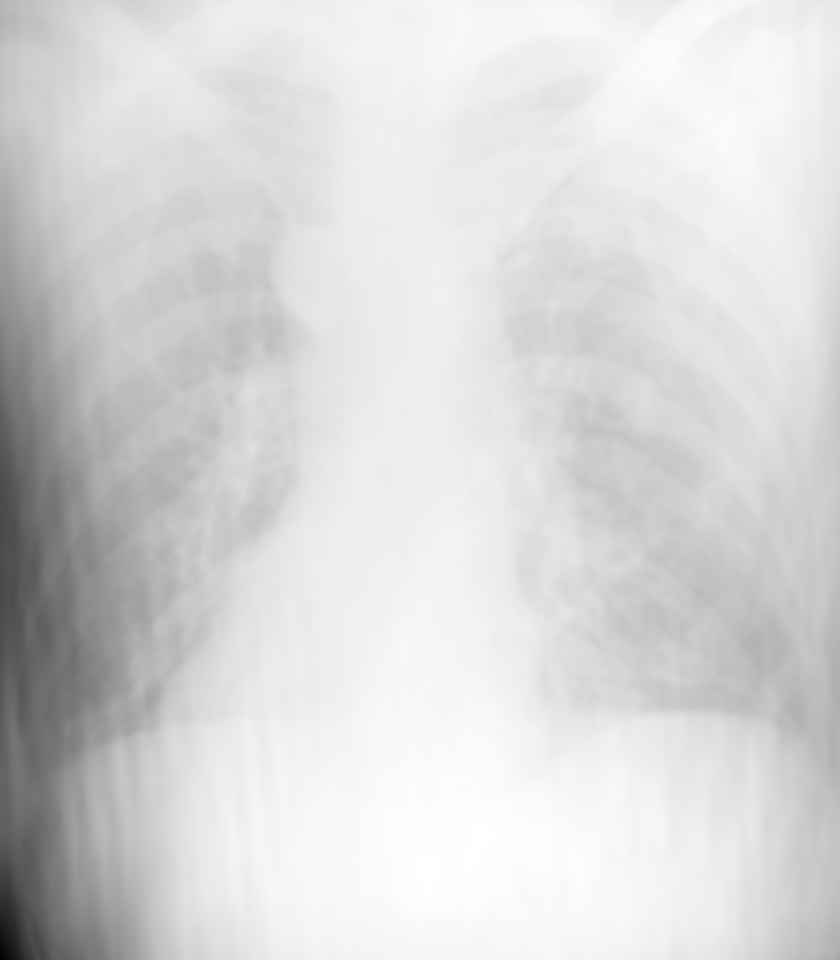}
            \caption{DeepDRR}
        \end{subfigure} \\
    \end{tabular}
    \caption{Simulated X-ray images with different components.}
    \label{fig:versus}
\end{figure}
