# Supplementary material for: XraySyn: Realistic View Synthesis From a Single Radiograph Through CT Priors
Source: arXiv:2012.02407 source file (2022-03-24)
Supplement: Supplementary file 11 [file supplemental_material_old.tex]

\section{Supplemental Material}


\subsection{Comparison of CT2Xray and DeepDRR}
\input{imgs/supplemental/versus}
\input{imgs/supplemental/tissue_weight}
While CT2Xray is inspired by DeepDRR, it is improved in many aspects in order to work on the task of X-ray view synthesis. Beyond the ability to propagate gradients, we show here the other aspects of improvements of CT2Xray, namely in speed and flexibility. 

The DeepDRR pipeline involves segmentation of a CT volume into three materials: bones, tissues, and air. Each material is forward projected to generate $t_{bone, tissue, air}$ and undergoes attenuation calculation. A CNN-based scatter estimation and a Poisson noise are added on top of the attenuation calculation. As shown in Fig. \ref{fig:versus}, we find that the scatter estimation CNN is not robust enough for general usage, and finetuning it requires MC simulation of X-ray images, which is infeasible to scale. Based on the results from DeepDRR, scatter estimation contributes relatively little to the overall image quality; therefore, we discard the scatter estimation. We also discard the calculation of $t_{air}$, as we find that the simulation without it bares more semblance to real X-ray images found in CheXpert, where the contrast between bone and air is significantly higher. Overall, CT2Xray is about five times faster than DeepDRR.


Since tissues consist of a wide range of materials, each with different attenuation rate, and the current CT2Xray pipeline considers all tissue as one material, there exists discrepancies between the generated X-ray image and a real X-ray image. Specifically, there is no way to modulate the contribution of $\mu_{tissue}$ in the final X-ray output when $\mu_{tissue}$ is either over-estimated or under-estimated. We therefore introduce a weight $\omega_{tissue}$ to fill this need. As shown in Fig. \ref{fig:tissue_weight}, when $\mu_{tissue}$ is clearly over-estimated for the heart region, we can lower $\omega_{tissue}$ to make it much more similar to the real X-ray input.
